# Supplementary material for: RESEARCHHUB: A Personalized Literature Discovery System for Biomedical Preprints
Source: arXiv:2610.28636 source file (2026-08-05)
Supplement: Supplementary file 1 [file evaluation_methods_additional.tex]

\section{Proposed Experimental Evaluation}

To systematically evaluate the dense retrieval recommender system, we can assess performance across four complementary dimensions:
(1) retrieval effectiveness,
(2) domain adaptation impact,
(3) interpretability faithfulness,
and (4) system-level performance.
The following experiments outline a comprehensive evaluation framework for the proposed architecture.

\subsection{Experimental Setup}

\paragraph{Corpus.}
We can evaluate the system on a corpus of MedRxiv preprints consisting of titles, abstracts, authors, and publication dates.
Each document can be represented as the concatenation of title and abstract.
Documents below a minimum length threshold (e.g., 50 characters) can be excluded to ensure meaningful representations.

\paragraph{Models.}
We can compare:
\begin{itemize}
    \item \textbf{Base Encoder:} \texttt{msmarco-distilbert-base-v3}.
    \item \textbf{Domain-Adapted Encoder:} The same architecture fine-tuned using Generative Pseudo Labeling (GPL).
\end{itemize}

\paragraph{Indexing.}
All embeddings can be $\ell_2$-normalized and indexed using FAISS with inner product similarity.
To analyze efficiency trade-offs, we can compare exact search (\texttt{IndexFlatIP}) with approximate search (\texttt{IndexIVFFlat}).

\subsection{Offline Retrieval Evaluation}

\paragraph{Query Construction.}
We can construct evaluation queries using:
\begin{itemize}
    \item Paper titles.
    \item First sentences of abstracts.
    \item Synthetic queries generated via GPL.
\end{itemize}

\paragraph{Relevance Definition.}
Relevance can be defined using topic-level alignment, where documents sharing the same inferred topic label are treated as relevant.
Alternatively, we can define relevance via biomedical keyword overlap or citation relationships if available.

\paragraph{Metrics.}
We can report:
\begin{itemize}
    \item Precision@k
    \item Recall@k
    \item Mean Reciprocal Rank (MRR)
    \item nDCG@k
\end{itemize}
All metrics can be averaged across queries.

\paragraph{Baselines.}
We can compare the dense retriever against:
\begin{itemize}
    \item BM25 sparse retrieval.
    \item Base SentenceTransformer.
    \item GPL fine-tuned SentenceTransformer.
\end{itemize}

\subsection{Ablation Studies}

To understand component contributions, we can evaluate:

\begin{itemize}
    \item \textbf{Embedding Normalization:} Remove $\ell_2$ normalization prior to indexing.
    \item \textbf{Domain Adaptation:} Compare base and GPL fine-tuned encoders.
    \item \textbf{Index Structure:} Compare exact and approximate FAISS indices.
    \item \textbf{Pseudo-Label Filtering:} Evaluate GPL training with and without cross-encoder filtering.
\end{itemize}

We can measure differences in nDCG@10 and latency to analyze accuracy--efficiency trade-offs.

\subsection{Domain Adaptation Analysis}

To assess domain specificity improvements, we can construct queries containing rare biomedical terminology (e.g., cytokine markers, molecular pathways, pharmacological targets).
We can then compare retrieval performance between the base and GPL-adapted models by analyzing:
\begin{itemize}
    \item Recall@10 for biomedical-specific queries.
    \item Topic coherence within top-k results.
    \item Qualitative relevance differences.
\end{itemize}

\subsection{Explainability Evaluation}

\paragraph{Faithfulness Test.}
To evaluate attribution quality, we can conduct token removal experiments:
\begin{enumerate}
    \item Compute Integrated Gradients (IG) attribution scores.
    \item Remove the top-$m$ most attributed tokens.
    \item Recompute similarity and measure score degradation.
\end{enumerate}

We can compare this with removing random tokens.
A larger similarity drop after removing high-attribution tokens would indicate faithful explanations.

\paragraph{Human Alignment Study.}
If domain experts are available, we can collect human ratings assessing:
\begin{itemize}
    \item Relevance of highlighted tokens.
    \item Clarity of explanation.
    \item Usefulness of explanations in understanding recommendations.
\end{itemize}

\subsection{Robustness Experiments}

\paragraph{Synonym Perturbation.}
We can replace biomedical terms with synonyms (e.g., ``heart attack'' $\rightarrow$ ``myocardial infarction'') and measure retrieval stability.

\paragraph{Noise Injection.}
We can introduce typographical errors or lexical perturbations to queries and evaluate performance degradation.

\paragraph{Out-of-Distribution Queries.}
We can evaluate retrieval using:
\begin{itemize}
    \item Clinical-style queries.
    \item Patient-oriented language.
    \item Grant-style technical descriptions.
\end{itemize}

\subsection{Bias and Representation Analysis}

To examine potential retrieval bias, we can analyze:
\begin{itemize}
    \item Topic distribution entropy within top-k results.
    \item Author frequency distribution compared to corpus-level statistics.
\end{itemize}

Such analyses can reveal whether high-frequency topics or prolific authors disproportionately dominate recommendations.

\subsection{System-Level Evaluation}

\paragraph{Latency.}
We can measure:
\begin{itemize}
    \item Query embedding time.
    \item FAISS search time.
    \item End-to-end API response latency (P50 and P95).
\end{itemize}

\paragraph{Scalability.}
We can evaluate system performance across increasing corpus sizes and measure:
\begin{itemize}
    \item Retrieval latency.
    \item Memory usage.
    \item Retrieval quality.
\end{itemize}

\paragraph{Interaction Simulation.}
To assess end-to-end usability, we can simulate multi-step interaction flows (search $\rightarrow$ similar papers $\rightarrow$ refinement) and measure topic coherence and drift across successive retrieval steps.

\subsection{Statistical Testing}

For comparative experiments, we can apply paired statistical tests (e.g., bootstrap resampling) to determine whether observed performance differences are statistically significant.
